# Supplementary material for: Self-referenced coherent diffraction x-ray movie of Angstrom- and femtosecond-scale atomic motion
Source: arXiv:1608.03039 ancillary file (2016-08-31)
Supplement: Supplementary file 1 [file Supplement4.pdf]

## Supplement 4: Simulations and data fits

A vibrational wavepacket simulation and a rotational dephasing simulation using the experimental parameters are presented. Additional information is provided about the  $\beta_2$  coefficient in Eq. 5.

### Vibrational wavepacket simulation

The probability density of the  $B$ -state wavepacket  $|\psi_B(R, t)|^2$  excited in this experiment is simulated in Figure S1. The principal differences from the experiment are (1) the model is carried out in the molecular frame so that rotational degrees of freedom are absent and the only relevant parameter is the internuclear separation  $R$  between the iodine atoms; (2) only the X and B state manifolds in  $I_2$  are included in the density matrix, so dissociation channels are absent in the simulation; and (3) the excitation is simulated as an idealized transform-limited pulse. The initial charge distribution is a 100° C thermal vibrational ensemble (Eqn.10). The pump in the model is a 50 fs (FWHM) Gaussian laser pulse with a central wavelength of 520 nm. A split-step method is used to propagate the density matrix in time.

This simulation reproduces the diffuse nature of the wavepacket seen at the outer turning points in Fig.3. In addition, the cusp-like “molecular canon” features at the outer turning point are seen in both the simulation and the experiment. B-state wavepacket oscillations are much more prominent in the simulation than in the experimental result in Fig.3 largely due to the absence of rotational degrees of freedom in the thermal state and the absence of subsequent rotational diffusion, as well as the finite resolution blurring in the experiment. Another factor may be the possible presence of chirp in the excitation pulse, which is not modeled in the simulation.

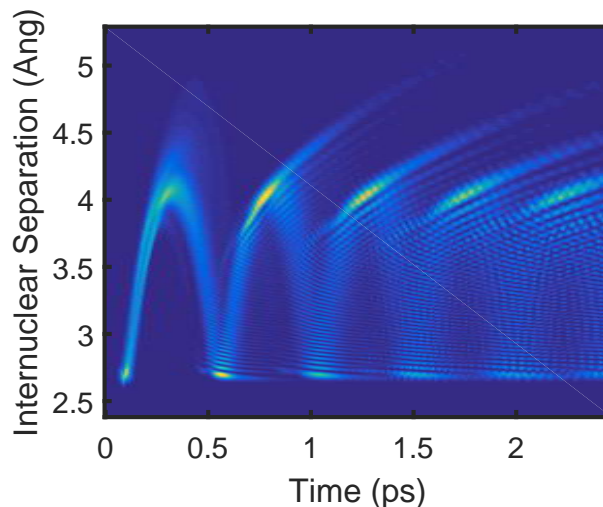

FIG. S1. Simulated vibrational wavepacket in  $I_2$  resulting from the interaction of a thermal (373 K) ground state with a 50 fs laser pulse with central wavelength 520 nm.

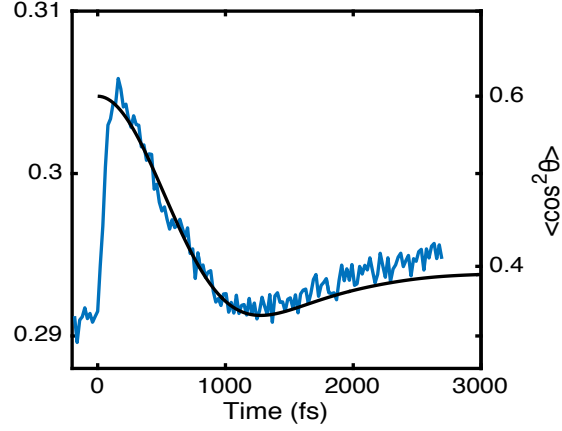

FIG. S2. The projection of Fig. 3 onto the time axis, i.e.  $\sum_Q \beta_2(Q, t)$  (blue, left axis). The black curve shows the calculated rotational dephasing of the thermal  $I_2$   $X$ -state impulsively projected into a  $\cos^2 \theta$  distribution (right axis).

### Rotational dephasing simulation

Figure S2 shows the projection of the  $\beta_2(Q, t)$  coefficient, shown in Fig.2, onto the  $Q$ -axis,  $\text{proj}_Q[\beta_2] = \sum_Q \beta_2(Q, t)$ . The decrease in the projection of the recorded data onto  $P_2(\cos^2 \theta)$  as a function of time, reaches a minimum near 1.2 ps. We attribute this decrease to rotational dephasing. The minimum in the signal near  $t = 1.2$  ps agrees quite well with previous measurements of rotational dephasing time as well as a model calculation of the rotational dephasing of a thermal  $X$ -state population projected onto a  $\cos^2 \theta$  distribution. The dephasing calculation is also shown in Fig. S2.

### Size of the $\beta_2$ coefficient

Figure S3 shows another representation of the  $\beta_2(Q, t)$  coefficient from Eqn.5. Here we show a very coarse time-series and do not perform any mean subtraction. One can see from the figure, that for almost all  $Q$ -values and times delays, the value of  $\beta_2$  is a positive value close to zero, indicating that the excitation is predominately due to a parallel electric-dipole transition, and the total projection of the data onto  $P_2(\cos \theta)$  is rather small. The fast  $Q$ -oscillations in the data below  $Q = 1.7 \text{ \AA}^{-1}$  we attribute to the heterodyne signal from the dissociating wavepacket. The heterodyne signal from the bound  $B$ -state wavepacket is seen as larger-period ( $T \sim 1.5 \text{ \AA}^{-1}$ )  $Q$ -oscillations beyond  $Q = 1.7 \text{ \AA}^{-1}$ .

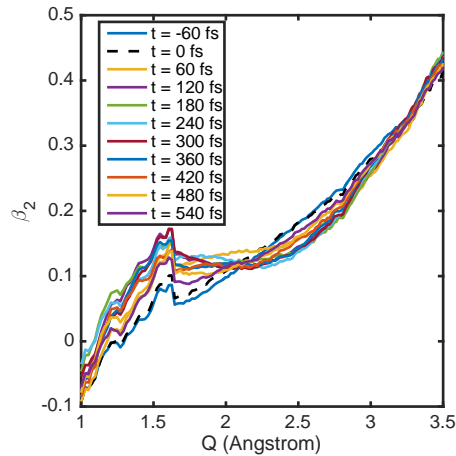

FIG. S3.  $\beta_2(Q, t)$  as defined in Eqn. ??, and shown in Fig ???. Here the data is shown without mean subtraction. The heterodyne signal for the  $B$ -state wavepacket can be seen in the long-period ( $\sim 1 \text{ \AA}^{-1}$ )  $Q$ -oscillations.
